# Supplementary material for: Novel Catchbond mediated oscillations in motor-microtubule complexes
Source: arXiv:2005.04600 source file (2020-07-13)
Supplement: Supplementary file 1 [file supplementary-july2020.pdf]

# Novel Catchbond mediated oscillations in motor-microtubule complex

# Supplementary Information

Sougata Guha,[1,2,*] Mithun K. Mitra,[1,†] Ignacio Pagonabarraga,[3,4,5,‡] and Sudipto Muhuri[2,§]

[1]*Department of Physics, Indian Institute of Technology Bombay, Mumbai, India*

[2]*Department of Physics, Savitribai Phule Pune University, Pune, India*

[3]*CECAM, Centre Européen de Calcul Atomique et Moléculaire, École Polytechnique Fédérale de Lasuanne (EPFL), Batochime, Avenue Forel 2, 1015 Lausanne, Switzerland*

[4]*Departament de Física de la Matèria Condensada, Universitat de Barcelona, Martí i Franquès 1, E08028 Barcelona, Spain*

[5]*UBICS University of Barcelona Institute of Complex Systems, Martí i Franquès 1, E08028 Barcelona, Spain*

(Dated: July 2, 2020)

## DIMENSIONLESS EQUATIONS AND FIXED POINTS

The dynamic equations of the system in terms of the scaled variables are given by,

$$\frac{d\tilde{l}}{d\tau} = -2\tilde{f}_s\Theta\left(n_c - \frac{N_p\zeta}{\tilde{l}}\right)\left[1 - \frac{N_p\zeta}{n_c\tilde{l}}\right] + \frac{2N_p\zeta\tilde{f}_s^{\,2}}{\tilde{l}\tilde{\Gamma}} \tag{1}$$

$$\frac{dn_c}{d\tau} = \gamma n_b - n_c\ \exp(\eta) \tag{2}$$

$$\frac{dn_b}{d\tau} = n_c\ \exp(\eta) - (1+\gamma)n_b + \Delta_n\left[\frac{\tilde{l}}{\tilde{f}_s} + 2\right] + 4\Delta_n\left[\frac{N_p\zeta\tilde{f}_s}{\tilde{l}\tilde{\Gamma}} - \Theta\left(n_c - \frac{N_p\zeta}{\tilde{l}}\right)\left(1 - \frac{N_p\zeta}{n_c\tilde{l}}\right)\right] \tag{3}$$

where,

$$\eta = \frac{N_p\zeta\tilde{f}_s}{n_c\tilde{l}\tilde{f}_d} - \Theta\left(\frac{N_p\zeta\tilde{f}_s}{n_c\tilde{l}} - \tilde{f}_m\right)\alpha\left[1 - \exp\left(-\frac{N_p\zeta\tilde{f}_s - n_c\tilde{l}\tilde{f}_m}{n_c\tilde{l}\tilde{f}_0}\right)\right]$$

The fixed points of Eqs. (1-3), $n_c^f, n_b^f, \tilde{l}^f$, must fulfill the constraint $n_c^f\tilde{l}^f > N_p\zeta$. They are determined by numerically solving the following equations simultaneously,

$$\Delta_n\gamma\left[\tilde{l}^f - 2\tilde{f}_s + \frac{4N_p\zeta\tilde{f}_s^2}{\tilde{l}^f}\left(\frac{1}{n_c^f\tilde{f}_s} + \frac{1}{\tilde{\Gamma}}\right)\right] = n_c^f\tilde{f}_s\ \exp(\eta^f) \tag{4}$$

$$\tilde{l}^f = N_p\zeta\tilde{f}_s\left(\frac{1}{n_c^f\tilde{f}_s} + \frac{1}{\tilde{\Gamma}}\right) \tag{5}$$

using $n_b^f = n_c^f\exp(\eta^f)/\gamma$, where $\eta^f = \eta(n_c^f, n_b^f, \tilde{l}^f)$.

## LINEAR STABILITY ANALYSIS

We perform a linear stability analysis about the fixed point to obtain the linear stability boundary separating regions of linearly stable overlap with the region for which the overlap is not linearly stable. A linear stability analysis about the fixed point yields an eigenvalue equation which has a cubic form,

$$\lambda^3 + a\lambda^2 + b\lambda + c = 0$$

Focusing on the case for which one of the eigenvalue is real and negative, the other two are complex conjugate, the linear stability boundary corresponds to the curve $c = ab$

which is obtained by making use of the fact that the real part of the complex conjugate pair of eigenvalues change sign at the linear stability boundary. By analyzing the change in behavior of the eigenvalues, the phase diagram that characterizes the different dynamical behaviour of the MT-motor complexes can be constructed. When the real part of all the eigenvalues are negative, the fixed point is linearly stable, and it corresponds to a region of stable overlap of the complex. Moving across the curve $c = ab$, the real part of the two of the complex conjugate eigenvalues, changes sign and consequently, separates a region of linear stable overlap with linearly unstable overlaps.

## EXPERIMENTAL PARAMETER VALUES

| **Parameter** | **Value** | **Parameter** | **Value** |
|---|---|---|---|
| $f_s$ | 1-7 pN [1–3] | $k_BT$ | 4.2 pN-nm |
| $v_0$ | 0.1 $\mu$m/s [3] | $f_d$ | 0.67 pN [4, 5] |
| $k_b$ | 1/s [6] | $f_0$ | 38.7 pN [4, 5] |
| $k_u^0$ | 1/s [7] | $\alpha$ | 68 [4, 5] |
| $\epsilon$ | $2k_BT$ [8] | $f_m$ | 1.4 pN [4, 5] |
| b | 1.3 nm [9] | $\Gamma$ | 10000 $k_BTs/\mu m^2$ [10] |

TABLE I. Characteristic magnitudes of the relevant model parameters that control the effective behavior of MT complexes. Relevant references is indicated next to each listed magnitude.

## VARIATION OF AMPLITUDE AND TIME PERIOD WITH $\tilde{f}_s$

We can also characterize the variation of the amplitude and the time period of the oscillations in this regime for different values of $f_s$. This is shown in Fig. 1 for a constant value of the parameter $\Delta_n$. The finite amplitude of the $n_c$ and the $\tilde{l}$ oscillations in the beginning of the limit cycle regions indicates that the bifurcation is sub-critical, reminiscent of first order phase transitions. The time period of the oscillations shows an asymmetric decrease in time period as we go deeper into the limit cycle region from the linear stability boundary. The time periods of the oscillations are roughly of the order of 1-10 seconds, and the amplitude

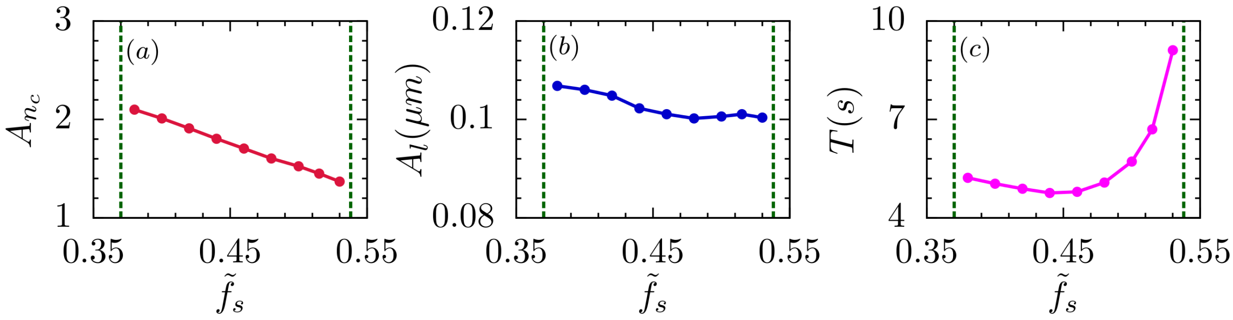


FIG. 1. Panel (a) and (b) shows the amplitude of oscillations of $n_c$ and $l$ respectively while panel (c) depicts the time period of limit cycle oscillations as a function of $\tilde{f}_s$ for $\Delta_n = 1.5$. The green dashed line denotes the limit cycle boundary for the particular set of parameters. All other parameters are same as Fig. 2(d) of main text.

of the overlap length oscillations are of the order of few hundred nanometers, both of which are consistent with observed biological estimates of amplitudes and time periods of spindle oscillations [11] as well as oscillations in myosin fibers [12].

## LIMIT CYCLE UNDER NOISE

In order to check the robustness of the limit cycle in noisy biological systems, we introduce a random stochastic noise in the dynamics for the overlap length.

$$\frac{dl}{dt} = -2v_0\ \Theta\ (n_c f_s - F_p) \left(1 - \frac{F_p}{n_c f_s}\right) + \frac{F_p}{\Gamma} + \sqrt{2D}\xi(t) \tag{6}$$

where $\xi(t)$ is the Gaussian white noise, $D = \frac{U}{\Gamma}$ which characterises noise strength and $U$ is the corresponding energy scale.

Therefore the dimensionless evolution equation of overlap length is given by,

$$\frac{d\tilde{l}}{d\tau} = -2\tilde{f}_s \Theta \left(n_c - \frac{N_p \zeta}{\tilde{l}}\right) \left[1 - \frac{N_p \zeta}{n_c \tilde{l}}\right] + \frac{2N_p \zeta \tilde{f}_s^{\,2}}{\tilde{l}\tilde{\Gamma}} + \sqrt{2\tilde{D}}\xi(t) \tag{7}$$

where $\tilde{D} = D \left(\frac{\tilde{f}_s}{v_0}\right)^2$.

Note that the coupling of the overlap length with the numbers of crosslinked and bound motors through the dynamical equations implies that the evolution of $n_c$ and $n_b$ also has a

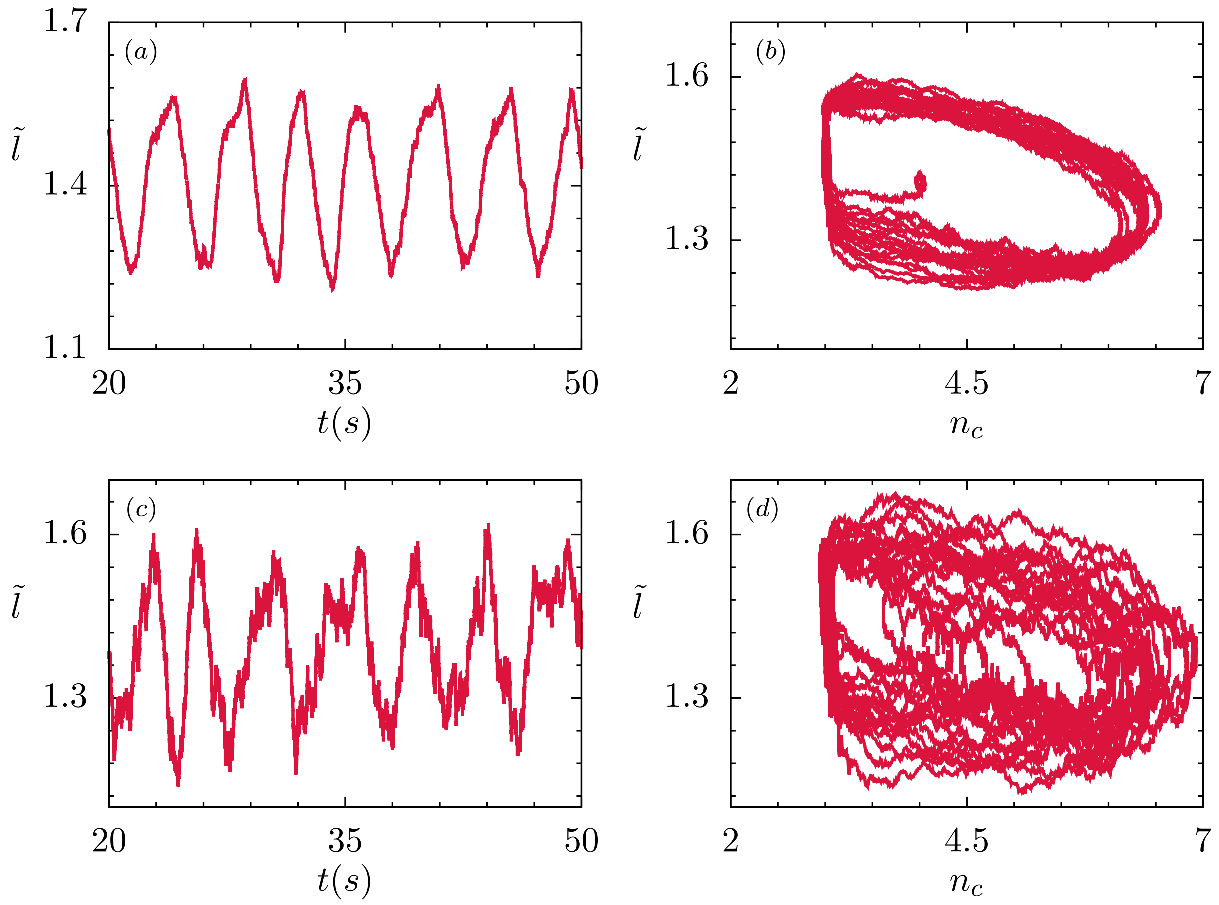


FIG. 2. Limit cycle oscillations in $\tilde{l}$-time plane (left panels) and in $\tilde{l} - n_c$ plane (right panels) when a Gaussian white noise is introduced only in the time evolution of overlap length (Eqn. 6). The values of diffusion coefficient are $D = 10^{-5}$ $\mu m^2/s$ (in (a) and (b)) and $D = 10^{-4}$ $\mu m^2/s$ (in (c) and (d)). All other parameter values are same as Fig. 3 of main text.

contribution from this noisy dynamics. We study the evolution of the dynamical equations for different values of noise strength ($D$). This is shown in Fig.2. For small noise values, $D = 10^{-5}\mu m^2/s$ ($U \sim 0.1\ k_BT$), the limit cycle oscillations persist, as is shown in Fig. 2(a) for the overlap length, and the only effect of the noise is to smear out the limit cycle boundary, as is shown in the $\tilde{l} - n_c$ plane in Fig. 2(b). Increasing the noise strength by an order of magnitude to $D = 10^{-4}\mu m^2/s$ ($U \sim k_BT$) further disrupts the oscillation, but the underlying limit cycle behaviour is still apparent in this case, as is shown in Fig. 2(c) and (d). Comparing with the binding energy scale of the passive crosslinkers, $\epsilon = 2k_BT$, we see that the limit cycle oscillations seen in this system are extremely robust even under

fluctuations of the order of the underlying energy scales in the system.

---


* sougataguha@iitb.ac.in

† mithun@phy.iitb.ac.in

‡ ipagonabarraga@ub.edu

§ sudipto@physics.unipune.ac.in



[1] R. Mallik, D. Petrov, S. Lex, S. King, and S. Gross, Current Biology **15**, 2075 (2005).

[2] S. Toba, T. M. Watanabe, L. Yamaguchi-Okimoto, Y. Y. Toyoshima, and H. Higuchi, Proceedings of the National Academy of Sciences **103**, 5741 (2006).

[3] V. Belyy, M. A. Schlager, H. Foster, A. E. Reimer, A. P. Carter, and A. Yildiz, Nature Cell Biology **18**, 1018 (2016).

[4] A. Kunwar, S. K. Tripathy, J. Xu, M. K. Mattson, P. Anand, R. Sigua, M. Vershinin, R. J. McKenney, C. Y. Clare, A. Mogilner, *et al.*, Proceedings of the National Academy of Sciences **108**, 18960 (2011).

[5] A. Nair, S. Chandel, M. K. Mitra, S. Muhuri, and A. Chaudhuri, Physical Review E **94**, 032403 (2016).

[6] C. Leduc, O. Campàs, K. B. Zeldovich, A. Roux, P. Jolimaitre, L. Bourel-Bonnet, B. Goud, J.-F. Joanny, P. Bassereau, and J. Prost, Proceedings of the National Academy of Sciences **101**, 17096 (2004).

[7] S. L. Reck-Peterson, A. Yildiz, A. P. Carter, A. Gennerich, N. Zhang, and R. D. Vale, Cell **126**, 335 (2006).

[8] S. Guha, S. Ghosh, I. Pagonabarraga, and S. Muhuri, EPL (Europhysics Letters) **124**, 58003 (2019).

[9] M. J. Schnitzer, K. Visscher, and S. M. Block, Nature Cell Biology **2**, 718 (2000).

[10] Z. Lansky, M. Braun, A. Lüdecke, M. Schlierf, P. R. ten Wolde, M. E. Janson, and S. Diez, Cell **160**, 1159 (2015).

[11] J. Pecreaux, J.-C. Röper, K. Kruse, F. Jülicher, A. A. Hyman, S. W. Grill, and J. Howard, Current Biology **16**, 2111 (2006).

[12] D. Sasaki, H. Fujita, N. Fukuda, S. Kurihara, and S. Ishiwata, Journal of Muscle Research and Cell Motility **26**, 93 (2005).
